# Supplementary material for: A variational approach to nucleation simulation
Source: arXiv:1808.04681 ancillary file (2018-08-14)
Supplement: Supplementary file 1 [file Piaggi-Valsson-Parrinello2016_SI.pdf]

# Supplementary information to "A variational approach to nucleation simulation"

Pablo M. Piaggi, Omar Valsson, and Michele Parrinello

Date: June 13th 2016

## 1 Comparison to metadynamics results

Since we are introducing a new methodology to calculate free energy surfaces of nucleation phenomena, we compare the results of the approach described in this work to a well-established technique, namely well-tempered metadynamics (WTmetaD)[1]. The comparison was made on a system of 864 atoms under the same thermodynamic conditions described in the main manuscript. As before, we measure all quantities in Lennard-Jones units[2], such that the Lennard-Jones well depth $\epsilon$ is the unit of energy and the Lennard-Jones diameter $\sigma_{LJ}$ is the unit of length. The details of the WTmetaD calculation are as follows. We employed the number of liquid-like atoms $n_l$ as CV (see main manuscript). The bias deposition stride was set to be 500 MD steps, the height of the kernels (gaussians) was set to 0.5 $\epsilon$ ($\sim 0.67$ $\mathrm{k_B T}$), and the width of the kernels was set to 1. A bias factor of 6 was employed, leading to barriers of $\sim 2$ $\mathrm{k_B T}$. We employed 4 multiple walkers in the calculation. In order to limit the sampling of CV space we introduced a static harmonic barrier:

$$V(s) = \begin{cases} 0 & \text{if } s < s_0 \\ \frac{1}{2}\kappa(s-s_0)^2 & \text{if } s > s_0 \end{cases}, \tag{S1}$$

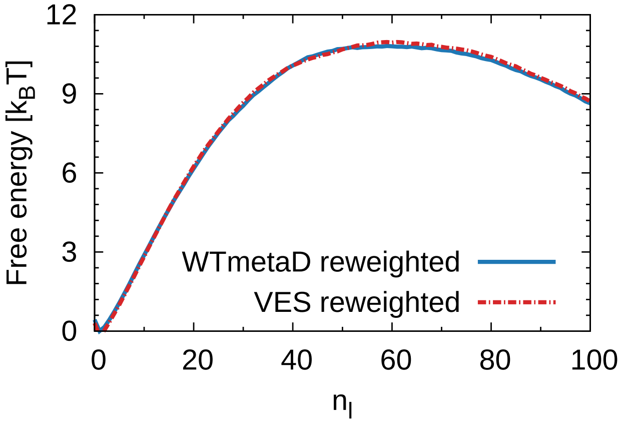


Figure S1: Reweighted free energy obtained from WTmetaD and the reweighted free energy obtained from the approach described in this work (VES).

with $s_0 = 150$ and $\kappa = 0.02$. The total simulation time per multiple walker was $5 \cdot 10^8$ MD steps. To obtain the free energy surface as a function of $n_l$ we could have exploited the fact that the WTmetaD potential converges asymptotically to[3]:

$$V(s,t) = -\left(1 - \frac{1}{\gamma}\right) F(s) + c(t) \tag{S2}$$

where $s$ is the biased CV. Instead, we employed a reweighting procedure[4] to obtain $F(n_l)$. This allows obtaining features of the free energy that WTmetaD kernels can not describe.

In Figure S1 we show a comparison of the reweighted free energy obtained from WTmetaD and the reweighted free energy obtained from the approach described in this work (VES). The two free energies agree within the statistical error. This provides a proof of the correctness of the approach described in the main manuscript.

# 2 Reweighting

In a simulation in the isothermal-isobaric ensemble, such as the ones carried out in this work, the statistical average of an observable $O(\mathbf{R})$ is:

$$\langle O(\mathbf{R})\rangle_{NPT} = \frac{\displaystyle\int d\mathbf{R}\, O(\mathbf{R})\, e^{-\beta[U(\mathbf{R})+PV]}}{Z_{NPT}} \tag{S3}$$

where $Z_{NPT}$ is the appropriate partition function. When a bias potential $V(s)$ is introduced, the statistical weight of each configuration $(\mathbf{R}, V)$ is altered and this must be taken into account in the calculation of ensemble averages. Henceforth, we shall drop the subscript $NPT$ to refer to the unbiased ensemble. In this way the equations will hold also if the simulations were performed in a different ensemble, e.g. the canonical ensemble. If the bias potential is static (time-independent), an average in the unbiased ensembled $\langle\cdot\rangle$ can be calculated from samples in the biased ensemble $\langle\cdot\rangle_V$ using[5]:

$$\langle O(\mathbf{R})\rangle = \frac{\langle O(\mathbf{R})\, \mathrm{e}^{\beta V(\mathbf{s}(\mathbf{R}))}\rangle_V}{\langle \mathrm{e}^{\beta V(\mathbf{s}(\mathbf{R}))}\rangle_V}. \tag{S4}$$

Given a simulation in which one has collected samples of the observable $O_1, ..., O_N$ and the corresponding bias potential $V_1, .., V_N$, the unbiased average of $O(\mathbf{R})$ is:

$$\langle O(\mathbf{R})\rangle = \frac{\sum_{i=1}^{N} O_i\, \mathrm{e}^{\beta V_i}}{\sum_{i=1}^{N} \mathrm{e}^{\beta V_i}}. \tag{S5}$$

In the variational approach, once $\Omega[V]$ has been minimized the bias potential becomes time-independent and thus equation (S4) can be used rigorously to calculate ensemble averages in the unbiased ensemble.

This formalism can be applied to the construction of a normalized histogram $N(s,t)$ of a collective coordinate $s$. The asymptotic value of $N(s,t)$ can be written as an ensemble average,

$$\lim_{t\to\infty} N(s,t) = P(s) = \langle \delta[s - s(\mathbf{R})] \rangle, \tag{S6}$$

with $P(s)$ the probability to observe a given value of the CV $s$. Therefore equation (S4) can be directly employed to calculate $N(s,t)$ in an biased simulation. In practice, instead of using $\delta[s - s(\mathbf{R})]$ one takes window functions $W(s, s_i, w)$ of width $w$ centered at $k$ points $s_i = s_1, ..., s_k$, with $s_i - s_{i-1} = w$. The normalized histogram can then be converted into a free energy employing the formula[3]:

$$F(s) = -\frac{1}{\beta} \lim_{t\to\infty} \log N(s,t). \tag{S7}$$

This is the procedure we have employed in this work to obtain the reweighted free energies as a function of $n_l$.

The cluster size distribution is intuitively defined as the average number of clusters of each size $n$. On more formal grounds, if $N_n(\mathbf{R})$ is the number of clusters of size $n$ for a given configuration $\mathbf{R}$, then the cluster size distribution can be rigurously defined as $\langle N_n \rangle$. Once that the cluster size distribution has been expressed as an ensemble average, it is possible to employ equation (S4) to calculate it from a biased simulation. We shall denote by $\overline{N_n}(t)$ the estimation at time $t$ of $\langle N_n \rangle$, and if the sampling is ergodic $\langle N_n \rangle = \lim_{t\to\infty} \overline{N_n}(t)$ holds. Then, a free energy $F(n)$ can be associated to the cluster size distribution using:

$$F(n) = -\frac{1}{\beta} \lim_{t\to\infty} \log \overline{N_n}(t). \tag{S8}$$

We point out that the cluster size distribution depends on the specific ensemble that is

used for the calculation[6]. In this work, the introduction of the barrier at $s_0$ leads to the constrained equilibrium ensemble envisioned in the classical theory of nucleation[6].

# 3 Collective variable

As described in the main manuscript, the bias potential $V(s)$ was constructed as a function of the total number of liquid-like atoms ($n_l$). In this section we provide details for the calculation of this CV.

We define $n_l$ as the number of atoms that have a coordination number larger than $c_0$ within a radius $r_0$. In order to use $n_l$ to construct the bias potential one needs to define it in a continuous and differentiable fashion. The calculation of $n_l$ can be thought of as divided in two stages. The first in which the coordination number of each atom is calculated as,

$$c_i = \sum_{j \,\in\, \text{neigh}} \frac{1 - \left(\frac{r_{ij}}{r_0}\right)^{12}}{1 - \left(\frac{r_{ij}}{r_0}\right)^{24}}, \tag{S9}$$

where $i$ is the atom index, $j$ runs over all neighbors of atom $i$, and $r_{ij}$ is the distance between atoms $i$ and $j$. In a second stage the number of atoms having a coordination number larger than $c_0$ is evaluated with:

$$n_l = \sum_{i \,\in\, \text{atoms}} \frac{1 - \left(\frac{c_i}{c_0}\right)^{-12}}{1 - \left(\frac{c_i}{c_0}\right)^{-24}}. \tag{S10}$$

For all the simulations we have employed $r_0 = 1.5$ and $c_0 = 4.5$.

# References


[1] A. Barducci, G. Bussi and M. Parrinello, *Physical review letters*, 2008, **100**, 020603.

[2] D. Frenkel and B. Smit, *Understanding molecular simulation: from algorithms to applications*, Academic press, 2001, vol. 1.

[3] O. Valsson, P. Tiwary and M. Parrinello, *Annual Review of Physical Chemistry*, 2016, **67**,.

[4] P. Tiwary and M. Parrinello, *The Journal of Physical Chemistry B*, 2014, **119**, 736–742.

[5] G. M. Torrie and J. P. Valleau, *Journal of Computational Physics*, 1977, **23**, 187–199.

[6] L. Maibaum, *Physical review letters*, 2008, **101**, 256102.
